# Supplementary material for: DiffFNO: Diffusion Fourier Neural Operator
Source: arXiv:2411.09911 source file (2025-04-05)
Supplement: Supplementary file 1 [file X_suppl.tex]

\clearpage
\setcounter{page}{1}
\maketitlesupplementary

% Sinuosidal embedding
\section{Time Embedding} \label{sec:time_embedding}

To effectively condition our neural network on the diffusion time step \( t \) during both training and inference, we incorporate a sinusoidal time embedding \( \mathbf{e}(t) \), inspired by positional encodings used in transformer architectures \cite{Attention}. This embedding captures temporal information across multiple frequencies, enabling the network to learn temporal dynamics at different scales. \( \mathbf{e}(t) \) is defined as:
\begin{equation}
\mathbf{e}(t) = \left[ \sin\left( \omega_1 t \right), \cos\left( \omega_1 t \right), \dots, \sin\left( \omega_D t \right), \cos\left( \omega_D t \right) \right],
\label{eq:time_embedding}
\end{equation}
where \( D \) is the dimensionality of the embedding (we set \( D = 64 \)), and the frequencies \( \omega_i \) are determined by an exponentially increasing schedule:
\begin{equation}
\omega_i = \omega_{\text{min}} \cdot \left( \frac{\omega_{\text{max}}}{\omega_{\text{min}}} \right)^{\frac{i-1}{D-1}}, \quad i = 1, 2, \dots, D,
\label{eq:frequency_schedule}
\end{equation}
with \( \omega_{\text{min}} = 1 \) and \( \omega_{\text{max}} = 10{,}000 \). This configuration ensures coverage of a wide range of frequencies, allowing the network to capture both rapid and slow temporal variations.

\( \mathbf{e}(t) \) is concatenated to the encoded image features \( \mathbf{v} \) obtained from the convolutional encoder. This enriched feature representation is then passed to both the \NewFNOLong (\NewFNOShort) and the \SpatialNOLong (\SpatialNOShort), ensuring that temporal information is available in subsequent processing stages.

By conditioning on the time step \( t \), the network can adapt its processing to different stages of the diffusion process. Early in the reverse diffusion (at higher \( t \)), the network focuses on reconstructing coarse structures from noisy inputs, while at later stages (lower \( t \)), it refines fine details. The sinusoidal time embedding facilitates this adaptation by providing a rich temporal context, enhancing the network's ability to model the evolution of image features over time.

This approach is consistent with recent practices in diffusion models \cite{DDPM, DPM-Solver}, where time embeddings play a crucial role in guiding the denoising process. Incorporating the time embedding directly into the network's input features allows \MethodShort to effectively leverage temporal information, contributing to its superior performance in arbitrary-scale super-resolution tasks.

% ODE Solver detail
\section{\NewSolverLong Update Step}
\label{sec:new_solver_update}
Our \NewSolverShort approach yields the adaptive time steps \(\{ t_i \}_{i=0}^N\), discretizing the ODE and apply a high-order solver for efficient and accurate sampling. The state of the system at each time step is updated using the Runge-Kutta 4th-order (RK4) method, which provides a good balance between computational efficiency and solution accuracy.

The general update equation for advancing from time \( t_i \) to \( t_{i+1} \) is given by:
\begin{equation}
\mathbf{x}_{i+1} = \mathbf{x}_i + h_i \cdot f_\theta(\mathbf{x}_i, t_i), \quad h_i = t_{i+1} - t_i,
\label{eq:update_equation}
\end{equation}
where \( \mathbf{x}_i \) is the estimate of the image \( \mathbf{x} \) at time \( t_i \), \( h_i \) is the adaptive step size, and \( f_\theta(\mathbf{x}_i, t_i) \) is the approximate drift function.

To achieve higher accuracy in solving the ODE, we employ the RK4 method. The update equations become:
\begin{align}
k_1 &= f_\theta(\mathbf{x}_i, t_i), \\
k_2 &= f_\theta\left(\mathbf{x}_i + \frac{h_i}{2} k_1, \, t_i + \frac{h_i}{2}\right), \\
k_3 &= f_\theta\left(\mathbf{x}_i + \frac{h_i}{2} k_2, \, t_i + \frac{h_i}{2}\right), \\
k_4 &= f_\theta\left(\mathbf{x}_i + h_i k_3, \, t_i + h_i\right), \\
\mathbf{x}_{i+1} &= \mathbf{x}_i + \frac{h_i}{6} (k_1 + 2k_2 + 2k_3 + k_4).
\label{eq:rk4_method}
\end{align}

Here, \( k_1, k_2, k_3, \) and \( k_4 \) are intermediate slopes evaluated at different points within the interval \( [t_i, t_{i+1}] \). The RK4 method effectively averages these slopes to compute a more accurate estimate of \( \mathbf{x}_{i+1} \).

% Implementation detail
\section{Implementation Details}
Low-resolution (LR) images are generated by downsampling 128×128 patches of high-resolution (HR) images using bicubic interpolation with random scaling factors uniformly sampled from ×1 to ×4. The patches acquired by uniform random sampling of all possible ways they could fit in the HR image. To enhance the robustness of our models to various transformations, we augment our data by applying random horizontal and vertical flips, as well as 90-degree rotations. We use a batch size of 64.

\textbf{Encoder (Lifting Layer)}. we used a both the Enhanced Deep Residual Networks (EDSR)'s baseline model and the larger Residual Dense Network (RDN) to extract rich features from the LR input.

\textbf{WFNO}. 8 layers, each with 64 channels and adaptive mode weighting applied to all frequency modes. In particular, features are intrinsically upsampled from LR to HR spatial dimensions through operations in the frequency domain.

\textbf{AttnNO}. 8 layers with 64 channels, employing single-head attention mechanisms. Features are upsampled via interpolation.

\textbf{Gated Fusion Mechanism}. Integrates features from WFNO and AttnNO using a 1×1 convolution followed by a sigmoid activation.

\textbf{AT-ODE Solver}. implements the Runge-Kutta (4,5) method with dynamic step size control based on local error estimation. Initial step size is set to to 1e-2, with a minimum step size of 1e-4. Absolute and relative error tolerances set to 1e-6.

During training, we use the Adam optimizer with $\beta_1=0.9$ and $\beta_2=0.999$. The learning rate is gradually increased from $1e-6$ to $3e-4$ over the first 5 epochs to stabilize training. A cosine annealing learning rate scheduler with warm restarts is employed. The learning rate then decreases from 3e-4 to 1e-6 following a cosine curve over each cycle of 50 epochs. We train our model over 1000 epochs total. We added an early-stopping mechanism to prevent model overfitting. Our loss function is the Mean squared error (MSE) between the predicted and true scores in the diffusion process. Experiments were conducted on a Linux server with an NVIDIA A100 GPU.

To increase data loading efficiency, we use 16 worker threads.

% Hyperparam analysis
% TODO: table showing the result of this analysis
\section{Hyperparameter Analysis}
We analyze the impact of key hyperparameters on model performance:
\begin{itemize}
    \item Number of Fourier Modes: Retaining all modes with adaptive weighting performs better than mode truncation. This highlights the importance of high-frequency components for the super-resolution task, and more importantly to adapt the architecture of neural operators to domains outside processes governed by physics laws or PDEs.
    \item Gating Mechanism Complexity: Increasing the depth of the gating network does not significantly improve results. On the one hand, this indicates that a simple 1×1 convolution suffices, which is good news for the computational cost of our DiffFNO architecture. On the other hand, this suggests that features learned in the frequency domain, which had benefited methods like LTE and HiNOTE, could complement featured learned in pixel space, such as through AttnNO in our method or SRNO. 
    \item Error Tolerance in AT-ODE: Setting tighter error tolerances improves PSNR but increases inference time marginally. A tolerance of 1e-6 balances quality and efficiency.
\end{itemize}

% TODO: qualitative results for different SR scales
\section{More Qualitative Results}
\newcommand{\matrixImgHeight}{3.2cm} % Adjusted height for each image in the 5x2 matrix
\newcommand{\matrixImgSpacing}{0.2cm} % Spacing between images
\newcommand{\largeImgHeight}{4.2cm} % Height for the enlarged GT image to match the height of the matrix

\begin{figure}[t]  % Use single-column 'figure'
  \centering
  \begin{tabular}{@{}c@{}}
    
    % GT image (X) on top
    \begin{tabular}{c}
      \includegraphics[height=\largeImgHeight]{sec/figures/qualitative/0839/0839_where.png} \\ % X image
      \small DIV2K Validation Set \cite{DIV2K}, $\times 7.6$
    \end{tabular} \\[0.3cm] % Add spacing between X and Y
    
    % 5x2 matrix (Y) below
    \begin{tabular}{
      c@{\hskip \matrixImgSpacing} c
    }
      % First row of the 5x2 matrix
      \includegraphics[height=\matrixImgHeight]{sec/figures/qualitative/0839/bicubic.png} &
      \includegraphics[height=\matrixImgHeight]{sec/figures/qualitative/0839/metasr.png} \\

      % Labels for first row
      \small Bicubic & \small Meta-SR \cite{SR-Meta-SR} \\

      % Second row of the 5x2 matrix
      \includegraphics[height=\matrixImgHeight]{sec/figures/qualitative/0839/lte.png} &
      \includegraphics[height=\matrixImgHeight]{sec/figures/qualitative/0839/liif.png} \\

      % Labels for second row
      \small LTE \cite{SR-LTE} & \small LIIF \cite{SR-LIIF} \\

      % Third row of the 5x2 matrix
      \includegraphics[height=\matrixImgHeight]{sec/figures/qualitative/0839/lit.png} &
      \includegraphics[height=\matrixImgHeight]{sec/figures/qualitative/0839/lmi.png} \\

      % Labels for third row
      \small LIT \cite{SR-LIT} & \small LMI \cite{SR-LMI} \\

      % Fourth row of the 5x2 matrix
      \includegraphics[height=\matrixImgHeight]{sec/figures/qualitative/0839/srno.png} &
      \includegraphics[height=\matrixImgHeight]{sec/figures/qualitative/0839/hinote.png} \\

      % Labels for fourth row
      \small SRNO \cite{SR-SRNO} & \small HiNOTE \cite{SR-HiNOTE} \\

      % Fifth row of the 5x2 matrix
      \includegraphics[height=\matrixImgHeight]{sec/figures/qualitative/0839/ours.png} &
      \includegraphics[height=\matrixImgHeight]{sec/figures/qualitative/0839/0839_crop.png} \\

      % Labels for fifth row
      \small DiffFNO (ours) & \small GT \\

    \end{tabular}
    
  \end{tabular}
\end{figure}

% another column
\begin{figure}[t]  % Use single-column 'figure'
  \centering
  \begin{tabular}{@{}c@{}}
    
    % GT image (X) on top
    \begin{tabular}{c}
      \includegraphics[height=\largeImgHeight]{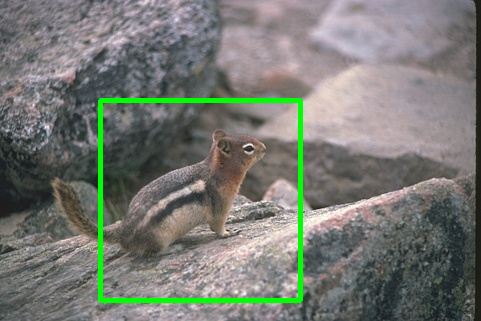} \\ % X image
      \small BSD100 \cite{BSD100}, $\times 3.2$
    \end{tabular} \\[0.3cm] % Add spacing between X and Y
    
    % 5x2 matrix (Y) below
    \begin{tabular}{
      c@{\hskip \matrixImgSpacing} c
    }
      % First row of the 5x2 matrix
      \includegraphics[height=\matrixImgHeight]{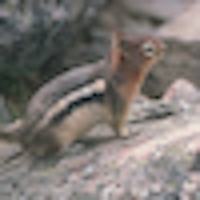} &
      \includegraphics[height=\matrixImgHeight]{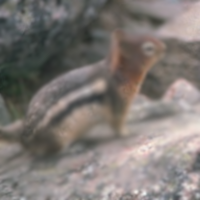} \\

      % Labels for first row
      \small Bicubic & \small Meta-SR \cite{SR-Meta-SR} \\

      % Second row of the 5x2 matrix
      \includegraphics[height=\matrixImgHeight]{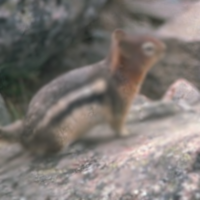} &
      \includegraphics[height=\matrixImgHeight]{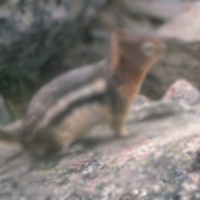} \\

      % Labels for second row
      \small LTE \cite{SR-LTE} & \small LIIF \cite{SR-LIIF} \\

      % Third row of the 5x2 matrix
      \includegraphics[height=\matrixImgHeight]{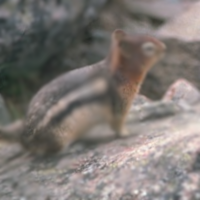} &
      \includegraphics[height=\matrixImgHeight]{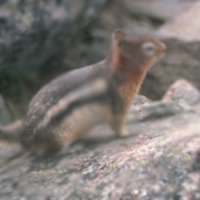} \\

      % Labels for third row
      \small LIT \cite{SR-LIT} & \small LMI \cite{SR-LMI} \\

      % Fourth row of the 5x2 matrix
      \includegraphics[height=\matrixImgHeight]{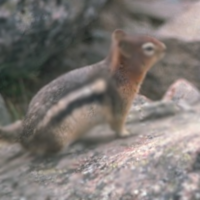} &
      \includegraphics[height=\matrixImgHeight]{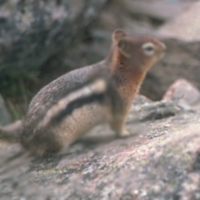} \\

      % Labels for fourth row
      \small SRNO \cite{SR-SRNO} & \small HiNOTE \cite{SR-HiNOTE} \\

      % Fifth row of the 5x2 matrix
      \includegraphics[height=\matrixImgHeight]{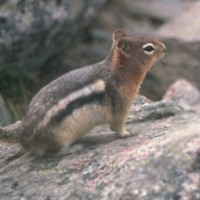} &
      \includegraphics[height=\matrixImgHeight]{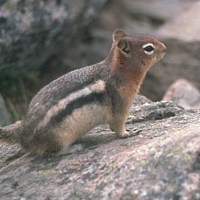} \\

      % Labels for fifth row
      \small DiffFNO (ours) & \small GT \\

    \end{tabular}
    
  \end{tabular}
\end{figure}

% column 3
\begin{figure}[t]  % Use single-column 'figure'
  \centering
  \begin{tabular}{@{}c@{}}
    
    % GT image (X) on top
    \begin{tabular}{c}
      \includegraphics[height=\largeImgHeight]{sec/figures/qualitative/Urban_082/urban100_082_where.png} \\ % X image
      \small Urban100 \cite{URBAN100}, $\times 11.2$
    \end{tabular} \\[0.3cm] % Add spacing between X and Y
    
    % 5x2 matrix (Y) below
    \begin{tabular}{
      c@{\hskip \matrixImgSpacing} c
    }
      % First row of the 5x2 matrix
      \includegraphics[height=\matrixImgHeight]{sec/figures/qualitative/Urban_082/bicubic.png} &
      \includegraphics[height=\matrixImgHeight]{sec/figures/qualitative/Urban_082/metasr.png} \\

      % Labels for first row
      \small Bicubic & \small Meta-SR \cite{SR-Meta-SR} \\

      % Second row of the 5x2 matrix
      \includegraphics[height=\matrixImgHeight]{sec/figures/qualitative/Urban_082/lte.png} &
      \includegraphics[height=\matrixImgHeight]{sec/figures/qualitative/Urban_082/liif.png} \\

      % Labels for second row
      \small LTE \cite{SR-LTE} & \small LIIF \cite{SR-LIIF} \\

      % Third row of the 5x2 matrix
      \includegraphics[height=\matrixImgHeight]{sec/figures/qualitative/Urban_082/lit.png} &
      \includegraphics[height=\matrixImgHeight]{sec/figures/qualitative/Urban_082/lmi.png} \\

      % Labels for third row
      \small LIT \cite{SR-LIT} & \small LMI \cite{SR-LMI} \\

      % Fourth row of the 5x2 matrix
      \includegraphics[height=\matrixImgHeight]{sec/figures/qualitative/Urban_082/srno.png} &
      \includegraphics[height=\matrixImgHeight]{sec/figures/qualitative/Urban_082/hinote.png} \\

      % Labels for fourth row
      \small SRNO \cite{SR-SRNO} & \small HiNOTE \cite{SR-HiNOTE} \\

      % Fifth row of the 5x2 matrix
      \includegraphics[height=\matrixImgHeight]{sec/figures/qualitative/Urban_082/ours.png} &
      \includegraphics[height=\matrixImgHeight]{sec/figures/qualitative/Urban_082/urban100_082_crop.png} \\

      % Labels for fifth row
      \small DiffFNO (ours) & \small GT \\

    \end{tabular}
    
  \end{tabular}
\end{figure}

% column 4
\begin{figure}[t]  % Use single-column 'figure'
  \centering
  \begin{tabular}{@{}c@{}}
    
    % GT image (X) on top
    \begin{tabular}{c}
      \includegraphics[height=\largeImgHeight]{sec/figures/qualitative/set5_bird/bird_where.png} \\ % X image
      \small Set5 \cite{SET5}, $\times 2.4$
    \end{tabular} \\[0.3cm] % Add spacing between X and Y
    
    % 5x2 matrix (Y) below
    \begin{tabular}{
      c@{\hskip \matrixImgSpacing} c
    }
      % First row of the 5x2 matrix
      \includegraphics[height=\matrixImgHeight]{sec/figures/qualitative/set5_bird/bicubic.png} &
      \includegraphics[height=\matrixImgHeight]{sec/figures/qualitative/set5_bird/metasr.png} \\

      % Labels for first row
      \small Bicubic & \small Meta-SR \cite{SR-Meta-SR} \\

      % Second row of the 5x2 matrix
      \includegraphics[height=\matrixImgHeight]{sec/figures/qualitative/set5_bird/lte.png} &
      \includegraphics[height=\matrixImgHeight]{sec/figures/qualitative/set5_bird/liif.png} \\

      % Labels for second row
      \small LTE \cite{SR-LTE} & \small LIIF \cite{SR-LIIF} \\

      % Third row of the 5x2 matrix
      \includegraphics[height=\matrixImgHeight]{sec/figures/qualitative/set5_bird/lit.png} &
      \includegraphics[height=\matrixImgHeight]{sec/figures/qualitative/set5_bird/lmi.png} \\

      % Labels for third row
      \small LIT \cite{SR-LIT} & \small LMI \cite{SR-LMI} \\

      % Fourth row of the 5x2 matrix
      \includegraphics[height=\matrixImgHeight]{sec/figures/qualitative/set5_bird/srno.png} &
      \includegraphics[height=\matrixImgHeight]{sec/figures/qualitative/set5_bird/hinote.png} \\

      % Labels for fourth row
      \small SRNO \cite{SR-SRNO} & \small HiNOTE \cite{SR-HiNOTE} \\

      % Fifth row of the 5x2 matrix
      \includegraphics[height=\matrixImgHeight]{sec/figures/qualitative/set5_bird/ours.png} &
      \includegraphics[height=\matrixImgHeight]{sec/figures/qualitative/set5_bird/bird_crop.png} \\

      % Labels for fifth row
      \small DiffFNO (ours) & \small GT \\

    \end{tabular}
    
  \end{tabular}
\end{figure}

% column 5
\begin{figure}[t]  % Use single-column 'figure'
  \centering
  \begin{tabular}{@{}c@{}}
    
    % GT image (X) on top
    \begin{tabular}{c}
      \includegraphics[height=\largeImgHeight]{sec/figures/qualitative/Urban100_03/urban100_03_where.png} \\ % X image
      \small Urban100 \cite{URBAN100}, $\times 6$
    \end{tabular} \\[0.3cm] % Add spacing between X and Y
    
    % 5x2 matrix (Y) below
    \begin{tabular}{
      c@{\hskip \matrixImgSpacing} c
    }
      % First row of the 5x2 matrix
      \includegraphics[height=\matrixImgHeight]{sec/figures/qualitative/Urban100_03/bicubic.png} &
      \includegraphics[height=\matrixImgHeight]{sec/figures/qualitative/Urban100_03/metasr.png} \\

      % Labels for first row
      \small Bicubic & \small Meta-SR \cite{SR-Meta-SR} \\

      % Second row of the 5x2 matrix
      \includegraphics[height=\matrixImgHeight]{sec/figures/qualitative/Urban100_03/lte.png} &
      \includegraphics[height=\matrixImgHeight]{sec/figures/qualitative/Urban100_03/liif.png} \\

      % Labels for second row
      \small LTE \cite{SR-LTE} & \small LIIF \cite{SR-LIIF} \\

      % Third row of the 5x2 matrix
      \includegraphics[height=\matrixImgHeight]{sec/figures/qualitative/Urban100_03/lit.png} &
      \includegraphics[height=\matrixImgHeight]{sec/figures/qualitative/Urban100_03/lmi.png} \\

      % Labels for third row
      \small LIT \cite{SR-LIT} & \small LMI \cite{SR-LMI} \\

      % Fourth row of the 5x2 matrix
      \includegraphics[height=\matrixImgHeight]{sec/figures/qualitative/Urban100_03/srno.png} &
      \includegraphics[height=\matrixImgHeight]{sec/figures/qualitative/Urban100_03/hinote.png} \\

      % Labels for fourth row
      \small SRNO \cite{SR-SRNO} & \small HiNOTE \cite{SR-HiNOTE} \\

      % Fifth row of the 5x2 matrix
      \includegraphics[height=\matrixImgHeight]{sec/figures/qualitative/Urban100_03/ours.png} &
      \includegraphics[height=\matrixImgHeight]{sec/figures/qualitative/Urban100_03/urban100_03_crop.png} \\

      % Labels for fifth row
      \small DiffFNO (ours) & \small GT \\

    \end{tabular}
    
  \end{tabular}
\end{figure}

% column 5
\begin{figure}[t]  % Use single-column 'figure'
  \centering
  \begin{tabular}{@{}c@{}}
    
    % GT image (X) on top
    \begin{tabular}{c}
      \includegraphics[height=\largeImgHeight]{sec/figures/qualitative/Urban100_099/urban100_99_where.png} \\ % X image
      \small Urban100 \cite{URBAN100}, $\times 8$
    \end{tabular} \\[0.3cm] % Add spacing between X and Y
    
    % 5x2 matrix (Y) below
    \begin{tabular}{
      c@{\hskip \matrixImgSpacing} c
    }
      % First row of the 5x2 matrix
      \includegraphics[height=\matrixImgHeight]{sec/figures/qualitative/Urban100_099/bicubic.png} &
      \includegraphics[height=\matrixImgHeight]{sec/figures/qualitative/Urban100_099/metasr.png} \\

      % Labels for first row
      \small Bicubic & \small Meta-SR \cite{SR-Meta-SR} \\

      % Second row of the 5x2 matrix
      \includegraphics[height=\matrixImgHeight]{sec/figures/qualitative/Urban100_099/lte.png} &
      \includegraphics[height=\matrixImgHeight]{sec/figures/qualitative/Urban100_099/liif.png} \\

      % Labels for second row
      \small LTE \cite{SR-LTE} & \small LIIF \cite{SR-LIIF} \\

      % Third row of the 5x2 matrix
      \includegraphics[height=\matrixImgHeight]{sec/figures/qualitative/Urban100_099/lit.png} &
      \includegraphics[height=\matrixImgHeight]{sec/figures/qualitative/Urban100_099/lmi.png} \\

      % Labels for third row
      \small LIT \cite{SR-LIT} & \small LMI \cite{SR-LMI} \\

      % Fourth row of the 5x2 matrix
      \includegraphics[height=\matrixImgHeight]{sec/figures/qualitative/Urban100_099/srno.png} &
      \includegraphics[height=\matrixImgHeight]{sec/figures/qualitative/Urban100_099/hinote.png} \\

      % Labels for fourth row
      \small SRNO \cite{SR-SRNO} & \small HiNOTE \cite{SR-HiNOTE} \\

      % Fifth row of the 5x2 matrix
      \includegraphics[height=\matrixImgHeight]{sec/figures/qualitative/Urban100_099/ours.png} &
      \includegraphics[height=\matrixImgHeight]{sec/figures/qualitative/Urban100_099/urban100_99_crop.png} \\

      % Labels for fifth row
      \small DiffFNO (ours) & \small GT \\

    \end{tabular}
    
  \end{tabular}
\end{figure}
